# Supplementary material for: Perturbation CheckLists for Evaluating NLG Evaluation Metrics
Source: arXiv:2109.05771 source file (2021-09-13)
Supplement: Supplementary file 1 [file additional_details.tex]

In particular, the preprocessing of the sentences370involves  a  combination  of  tokenization,  part-of-371speech tagging, named entity recognition, etc. The372targeted part of the sentence is then modified ei-373ther by leveraging simple string manipulation func-374tions  or  by  masking  and  generating  the  words/375phrases using the predictions by RoBERTa (Liu376et al., 2019).  For example, the application of the377template for ‘dropping stop words’ involves the378tokenization of the sentence using the NLTK word379tokenizer as the first step. The list of tokens is com-380pared with the set of stopwords provided by NLTK381to filter out the stop words from the list of tokens.382The modified sentence is then reconstructed using383the string join function by iterating over the tokens384in the modified list.   Similarly,  for the template385of ‘changing the attributes’ in case of image cap-386tioning, the sentence is first tokenized, then the ad-387jectives are identified using part-of-speech tagging388(again a functionality provided by NLTK). The list389of ‘related words’ (i.e., hyponyms of hypernyms390or ‘sibling words’) are obtained using WordNet391framework.  Unless the list returns empty, one of392the entries in the list is used to replace the origi-393nal adjective.  In order to ‘change question to an394assertive statement’, the question words (such as395who, what, why, when, etc) are replaced with a396‘mask’ token and the ‘?’ character at the end is re-397placed with ‘.’ using string replace function. This398modified sentence is fed to RoBERTa model which399generates different predictions to be used in place400of the ‘mask’ token. One of the suggested words401is  used  to  form  the  modified  assertive  sentence.402(Additional checks are made to ignore any bad sug-403gestiongs for this task such as question words /stop404word suggestion
